# Supplementary material for: Kyrix-S: Authoring Scalable Scatterplot Visualizations of Big Data
Source: arXiv:2007.15904 source file (2020-07-31)
Supplement: Supplementary file 1 [file appendix.tex]

There is a fairly rich literature of \visname-related systems. We include in this appendix a comprehensive comparison of \sys to existing systems, which complements Sections \ref{sec:introduction} and \ref{sec:relatedwork}. 

\section{A Tabular Comparison}
Table \ref{tab:featurecomparisondetailed} shows a detailed comparison of authoring systems for \visnames. We include 21 systems as subrows, and 9 detailed features as subcolumns. Check marks are used to indicate that a system has the corresponding feature. 

We can use this table to illustrate the claims we have made on the limitations of existing systems:
\begin{itemize}
\vspace{-.5em}
    \item \textbf{Both general pan/zoom systems and specialized \visname systems have limited scalability}. We can see from the \textit{Scalability} column that only four systems can support data beyond memory size, and only Perrot et al.\cite{perrot2015large} scales to billion-object scatterplots.
\vspace{-.5em}
    \item \textbf{General pan/zoom systems incur too much developer work}. As can be seen, none of the general pan/zoom systems support declarative authoring in 10s of lines of specifications. Also, all of them put the burden of mark layout generation on the developers. Specialized \visname systems, in contrast, mostly provide a concise authoring interface and all have an automatic layout generator.
\vspace{-.5em}
    \item \textbf{Specialized SSV systems have low flexibility}. As Table \ref{tab:featurecomparisondetailed} shows, none of the specialized \visname systems support all features under ``Expressivity \& Usability''. In fact, the number of such features supported by any specialized \visname system is at most three (Guo et al.\cite{guo2018efficient}, Kefaloukos et al.\cite{kefaloukos2014declarative} and Splatterplots\cite{mayorga2013splatterplots}). In particular, every specialized \visname system is focused on very specific visual marks, as indicated by the empty ``arbitrary mark types'' column. The inflexible nature of these systems makes it hard to extend them to general scenarios. 
\end{itemize}

\sys, on the other hand, supports all features. 

\section{Discussion on Layout Generators}
The layout generator in \sys decides how marks are placed on each zoom level, and serves as the key component to make \sys scale to big datasets. As discussed briefly in Section \ref{subsec:related_specialized}, \sys's layout generator is algorithmically similar in some ways to the ones in existing systems, but also significantly different in many aspects due to the broader design requirements. 

Here, we expand the discussion in Section \ref{subsec:related_specialized} to elaborate how \sys's layout generator compares to existing ones.

\vspace{.3em}
\subhead{Offline vs. online}. Some systems\cite{guo2018efficient,drosou2012disc,nutanong2012multiresolution} use an online approach which computes the layout of visual marks on the fly as user's viewport changes. Although being more amenable to updating data, this approach has two inherent drawbacks. First, it is susceptible to data skew as it often needs to iterate through a great portion, if not all of the objects in the viewport. In our examples, there can be tens of millions of objects in a viewport which would make these system unable to respond within 500ms (\textbf{G4-b}). Second, these systems cannot support aggregation-based marks (e.g. pie or bar) because without any precomputed indexes, computing the aggregation statistics requires going through all data in the current viewport. As shown in Table \ref{tab:featurecomparisondetailed}, none of \cite{guo2018efficient,drosou2012disc,nutanong2012multiresolution} can show aggregation information. In contrast, \sys precomputes the mark layouts offline, which makes it possible to support aggregation marks and respond to user interactions under 500ms despite data skew. 

% \vspace{.3em}
% \subhead{Data cube approaches}. Nanocubes\cite{lins2013nanocubes} and Hashedcubes\cite{pahins2016hashedcubes} use a data cube approach which precomputes all aggregation stats over every possible combination of dimensions. By using memory sharing techniques, these systems are able to deal with data that does not fit in memory. However, the biggest drawback of the data cube approach is that it does not support inspection of individual objects, which would require the system to store all objects that belong to a given combination of dimensions instead of just one number, essentially increasing the memory footprint by several orders of magnitude. 

\vspace{.3em}
\subhead{Greedy-based hierarchical sampling/clustering}. \sys's single-node layout algorithm is inspired by prior systems\cite{guo2018efficient,chen2014visual,kefaloukos2014declarative,perrot2015large}. Specifically, the basic algorithmic flow of iterating over all objects in importance order and then maintaining a minimum distance between objects is drawn from those systems. Nevertheless, \sys' goes two steps further by 1) generalizing this algorithmic framework to support more usability requirements (last three columns of Table \ref{tab:featurecomparisondetailed}), and 2) using spatial partitioning techniques to extend the algorithm to support scatterplots of billions of objects (Section \ref{subsec:multinodealgo}). 

% online vs offline -- offline is needed for skew & aggregation

% data cubes: narrower focus, not extendable to general scenarios

% common: a greedy algorithm, enforce an importance order, and minimal distance
% our difference is that we extend it to large scale using spatial partitioning

\setlength{\dashlinedash}{0.5pt}
\setlength{\dashlinegap}{4pt}

\begin{table*}[h]
%\centering
\vspace{-45em}
\caption{A tabular comparison of systems/toolkits for authoring \visnames.}
\label{tab:featurecomparisondetailed}
\resizebox{\textwidth}{!}{%
\begin{tabular}{|c|c|cc|cc|ccccc|}
\hline
\multicolumn{2}{|c|}{\multirow{2}{*}{}} & \multicolumn{2}{c|}{Scalability} & \multicolumn{2}{c|}{Authoring Capability} & \multicolumn{5}{c|}{Expressivity \& Usability} \\ \cline{3-11} 
\multicolumn{2}{|c|}{} & \begin{tabular}[c]{@{}c@{}}Support data\\ that cannot fit\\ in memory\end{tabular} & \begin{tabular}[c]{@{}c@{}}Distributed architecture\\ (billion-object\\ scalability)\end{tabular} & \begin{tabular}[c]{@{}c@{}}Declarative\\ authoring in 10s of\\ lines of code\end{tabular} &
\begin{tabular}[c]{@{}c@{}}Automatic\\ layout\\ generation\end{tabular} & 
\begin{tabular}[c]{@{}c@{}}Inspection\\ of important\\ objects\end{tabular} &
\begin{tabular}[c]{@{}c@{}}Arbitrary\\ mark\\ types\end{tabular} &
\begin{tabular}[c]{@{}c@{}}Show\\ aggregation\\ information\end{tabular} &
\begin{tabular}[c]{@{}c@{}}Support both\\ partial \&\\ non-overlap\end{tabular} &
\begin{tabular}[c]{@{}c@{}}Automatic\\ bounded visual\\ density\end{tabular} \\ \hline

Our work & \sys & \checkmark & \checkmark & \checkmark & \checkmark & \checkmark & \checkmark & \checkmark & \checkmark & \checkmark \\ \hline
\multirow{4}{*}{\begin{tabular}[c]{@{}c@{}}General\\ pan/zoom\\ systems\end{tabular}} & \textsf{Kyrix}\cite{tao2019kyrix} & \checkmark &  &  &  & \checkmark & \checkmark & \checkmark & \checkmark &  \\ \cdashline{2-11}
 & \textsf{Pad++}\cite{bederson1994pad++} &  &  &  &  & \checkmark & \checkmark & \checkmark & \checkmark &  \\ \cdashline{2-11}
 & \textsf{Jazz}\cite{bederson2003jazz} &  &  &  &  & \checkmark & \checkmark & \checkmark & \checkmark &  \\ \cdashline{2-11}
 & \textsf{ZVTM}\cite{pietriga2005toolkit} &  &  &  &  & \checkmark & \checkmark & \checkmark & \checkmark &  \\ \hline
\multirow{16}{*}{\begin{tabular}[c]{@{}c@{}}Specialized\\ \visname systems\end{tabular}} & \textsf{Cartolabe}\cite{cartolabe} &  &  &  & \checkmark & \checkmark &  & \checkmark &  &  \\ \cdashline{2-11}
 & \textsf{Leaflet}\cite{leafletcluster} &  &  & \checkmark & \checkmark &  &  & \checkmark &  & \checkmark \\ \cdashline{2-11}
 & Beilschmidt et al.\cite{beilschmidt2017linear} &  &  &  & \checkmark &  &  & \checkmark &  &  \\ \cdashline{2-11}
 & Chen et al.\cite{chen2014visual} &  &  & \checkmark & \checkmark &  &  &  & \checkmark & \checkmark \\ \cdashline{2-11}
 & Sarma et al.\cite{das2012efficient} &  &  & \checkmark & \checkmark & \checkmark &  &  &  & \checkmark \\ \cdashline{2-11}
 & Delort et al.\cite{delort2010vizualizing} &  &  &  & \checkmark &  &  & \checkmark &  &  \\ \cdashline{2-11}
 & Derthick et al.\cite{derthick2003constant} &  &  & \checkmark & \checkmark & \checkmark &  & \checkmark &  &  \\ \cdashline{2-11}
 & \textsf{Disc}\cite{drosou2012disc} &  &  &  & \checkmark & \checkmark &  &  & \checkmark &  \\ \cdashline{2-11}
 & Guo et al.\cite{guo2018efficient} &  &  &  & \checkmark & \checkmark &  &  & \checkmark & \checkmark \\ \cdashline{2-11}
 & Kefaloukos et al.\cite{kefaloukos2014declarative} &  &  & \checkmark & \checkmark & \checkmark &  &  & \checkmark & \checkmark \\ \cdashline{2-11}
 & Lekschas et al.\cite{lekschas2019pattern} &  &  &  & \checkmark & \checkmark &  & \checkmark &  &  \\ \cdashline{2-11}
 & \textsf{Nanocubes}\cite{lins2013nanocubes} & \checkmark &  & \checkmark & \checkmark &  &  & \checkmark &  &  \\ \cdashline{2-11}
 & \textsf{Splatterplots}\cite{mayorga2013splatterplots} &  &  & \checkmark & \checkmark & \checkmark &  & \checkmark &  & \checkmark \\ \cdashline{2-11}
 & Nutanong et al.\cite{nutanong2012multiresolution} &  &  & \checkmark & \checkmark & \checkmark &  &  & \checkmark &  \\ \cdashline{2-11}
 & \textsf{Hashedcubes}\cite{pahins2016hashedcubes} & \checkmark &  & \checkmark & \checkmark &  &  & \checkmark &  &  \\ \cdashline{2-11}
 & Perrot et al.\cite{perrot2015large} & \checkmark & \checkmark & \checkmark & \checkmark &  &  & \checkmark &  &  \\ \hline
\end{tabular}%
}
\end{table*}
